# Supplementary material for: For high-dimensional hierarchical models, consider exchangeability of effects across covariates instead of across datasets
Source: arXiv:2107.06428 source file (2021-07-13)
Supplement: Supplementary file 1 [file related_stat_gen.tex]

\subsection{Related Work in Statistical Genetics}\label{sec:related_stat_gen}

Many of methods in existing work in this area are driven by simplifications needed for computational reasons.
\begin{enumerate}
\item{requiring complete sample overlap, or imputing missing values as a first step}
\item{Requiring noise covariance to be the same as prior covariance.}
\end{enumerate}

\BLT{Add pithy summary about these being special case of exch. cov. effects.}

A number of recent works in statistical genetics consider models which address covariance of covariate effects corresponding to SNPs.

% Joint analysis of psychiatric disorders increases accuracy of risk prediction for Schizophrenia, Bipolar Disorder, and Major Depressive Disorder
% Maier, …., S. H. Lee, 2015 AJHG
\citet{maier2015joint} consider the problem of jointly modeling multiple psychiatric disorders to increase the accuracy of risk prediction. 
The authors motivate their approach with the potential increases in statistical efficiency that could be obtained by considering related traits, remarking in particular that by jointly modeling multiple disorders they can effectively increase their sample-sizes.
The authors acknowledge that with datasets available at the time of writing, their risk predictors are not clinically useful but remain a valuable research too.
\BLT{I find the statement of their linear mixed model to be very confusing.  In particular, I think parsing some of their notation requires a degree of familiarity with the related literature, as they do not define all of their notation.}

% Estimation of Pleiotropy between complex diseases
% S.H. Lee, … N.R. Wray, 2012 Bioinformatics
\citet{lee2012estimation} propose to use a bivariate linear mixed model to estimate the extent of pleiotropy (the involvement of genes in multiple phenotypes).
Their approach seems to assume a single population in which both phenotypes are observed, but does not allow for correlation in the noise.
\BLT{
    The main text of this paper is only two pages long, and the supplementary materials provide no additional clarification on the method.
Overall I have been unsuccessful in understanding the model they propose and their approach to inference (for example, I'm unsure of what some variables represent, and even of their dimensions).
The authors use an `average information' algorithm, which I'm unfamiliar with.
The paper was released with a \href{cnsgenomics.com/software/gcta/\#BivariateGREMLanalysis}{software package}.}

% ``Genetic relationship between five psychiatric disorders estimated from genome-wide SNPs''
% Cross-Disorder Group of the Psychiatric Genomics Consortium, 2013 Nature Genetics
Many of the same authors of \citet{lee2012estimation}, have applied this approach to examining the genetic correlation between several psychiatric disorders with the goal of understanding shared disease etiology among psychiatric traits\citep{lee2013genetic}.
The paper gives little explanation of the computational methods used, referencing their use of the approach of \citet{lee2012estimation}.
In this case, however, the cohorts for the studies in the different diseases appear to be disjoint.

% An atlas of genetic correlations across human diseases and traits
% B. Bulik-Sullivan, H. K. Finucane ... A. L. Price, B. M. Neal, 2015 Nature Genetics
\citet{bulik_finucane2015atlas} consider a model of several phenotypes similar to the model discussed in \Cref{sec:intro}, but without the restriction to exactly overlapping samples, 
and address the question of inferring the covariance in SNP effect sizes as an object of interest in its own right.
Their approach relies only on published summary statistics from association studies of different traits and uses a moment based estimator.
As the simplest form of their proposed estimator exhibits high variance, the authors use several techniques to reduce variance --  the ultimate estimates of the covariances have relative standard errors on the order of 20\% (computed with jackknife).
The authors do not address prediction.
%Methods for reducing variance:
%  - Multiple stages of estimation (Estimating intercept term, i.e. noise, with the outlier SNPs removed, and then estimating just the genetic correlation terms)
%  - Single trait LDSC to estimate some parameters
%  - Estimate variances to weight estimates in the regression (weighted least squares) 

% Multi-trait analysis of genome-wide association summary statistics using MTAG
% P. Turley, ..., D. J. Benjamin, 2018 Nature Genetics
\citet{turley2018multi} propose to jointly model the marginal effect sizes of SNPs across multiple traits to increase power to identify associations.
To this end they place a multivariate Gaussian prior on population marginal associations and use a moment based method to estimate the prior covariance.
Their modeling approach is distinct from ours in that they do not directly model prior correlation in the parameters a full multiple regression model across traits. 
The authors do not consider prediction.
%prior on marginal betas (avoids working with the regression problem by considering marginal association as estimand )
% Issue with non-pd matrices! In particular we can get a non pd estimate of $\Sigma_\beta$, which

% Efficient multivariate linear mixed model algorithms for genome-wide association studies
% Xiang Zhou and Mathew Stephens, Nature methods 2014
\citet{zhou2014efficient} geared towards identifying associations.
Describe an EM algorithm for fitting mixed effects model.
They do not discuss parameter inference.
Require complete sample overlap. \footnote{\BLT{check this.}}
Plos One paper by Stephens \citep{stephens2013unified} talks more about parameter inference -- summarize theory -- restricts to assumption on same noise variance and prior variance, same designs.
While this is reasonable in some settings (potentially GWAS with complete sample overlap), it is less appropriate in cases where samples corresponding to each regression problem are non-overlapping.
This work does not address exchangeabilty as a motivation for this class of priors.
