# Supplementary material for: For high-dimensional hierarchical models, consider exchangeability of effects across covariates instead of across datasets
Source: arXiv:2107.06428 source file (2021-07-13)
Supplement: Supplementary file 2 [file supp_aggregate_applications.pdf]

Blog Popularity

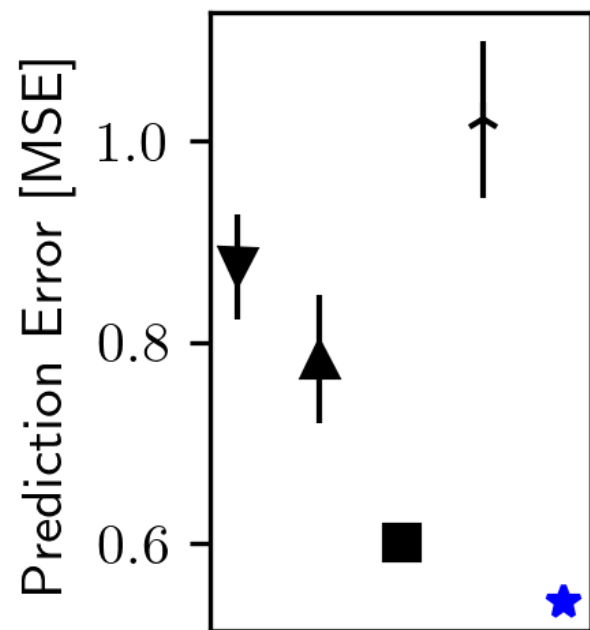

Law Enforcement

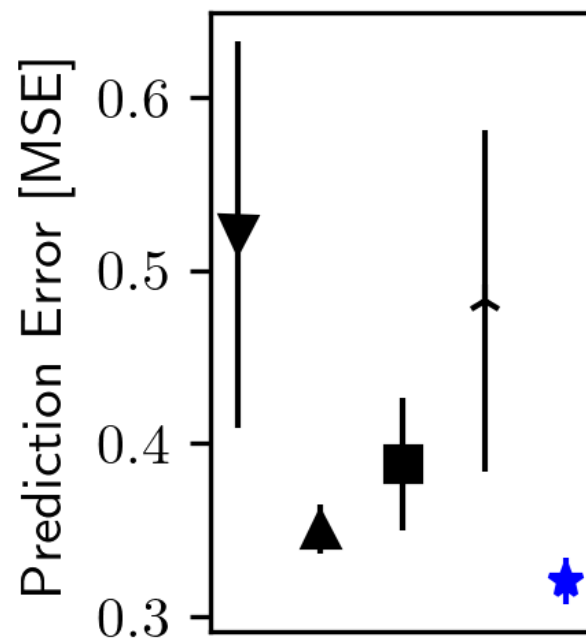

CIFAR10

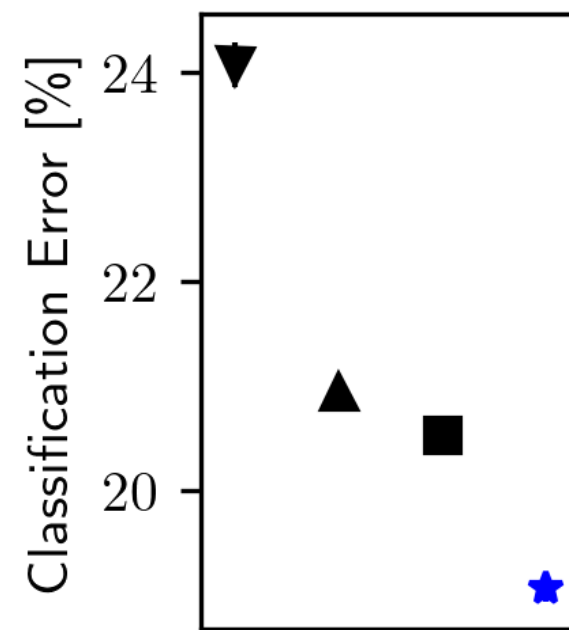

- Least Sqr./MLE
- Least Sqr./MLE Pool
- Indep. Bayes.
- Exch. Reg.
- Exch. Cov.**

Blog Popularity

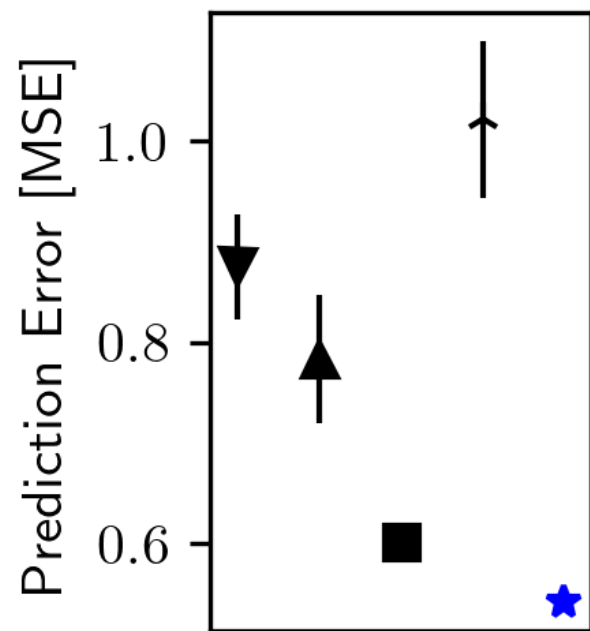

Law Enforcement

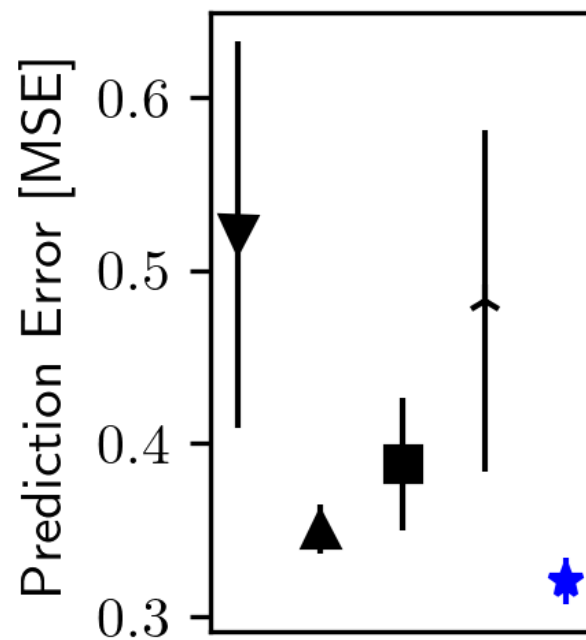

CIFAR10

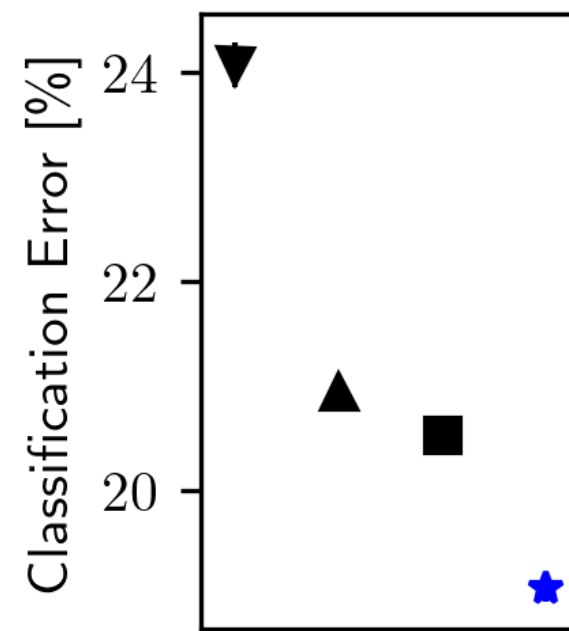

- ▼ Least Sqrs./MLE
- ▲ Least Sqrs./MLE Pool
- Indep. Bayes.
- ↑ Exch. Data
- ★ **Exch. Cov.**

# Law Enforcement

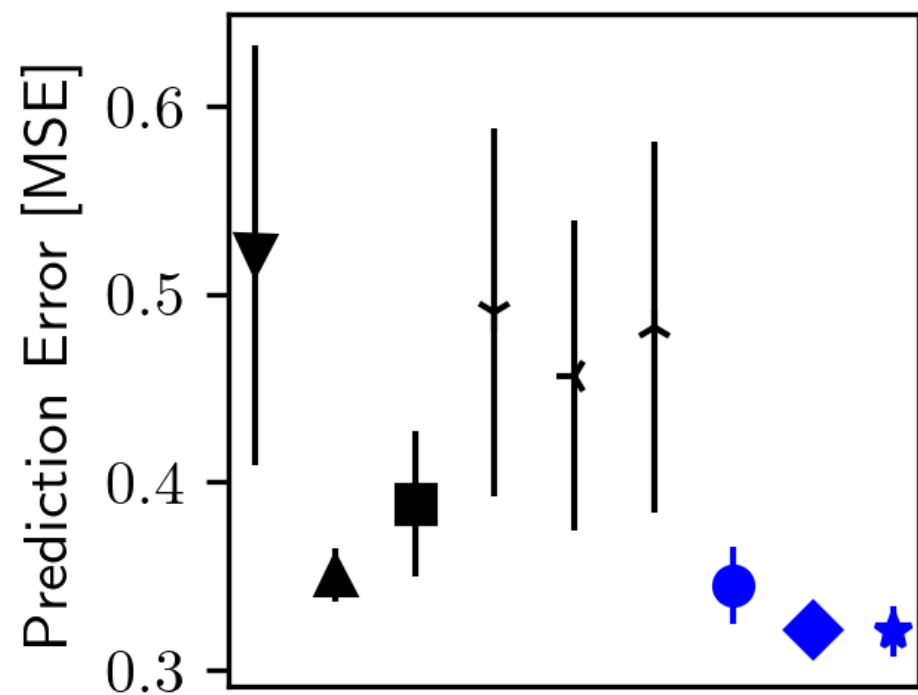

# Blogs

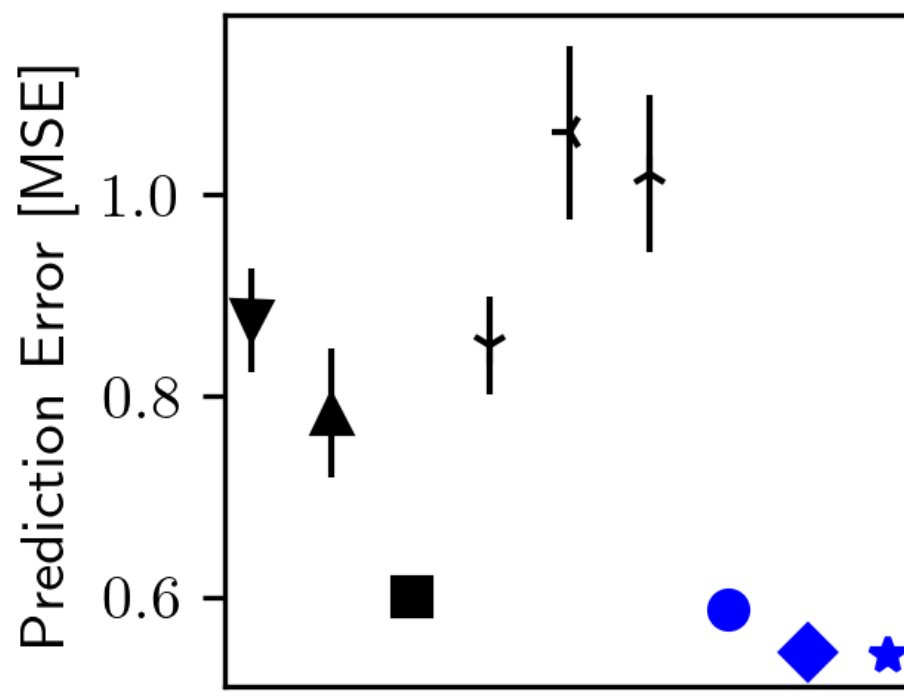

- ▼ Least Sqr./MLE
- ▲ Least Sqr./MLE Pool
- Indep. Bayes.
- ⋈ Exch. Reg. MM
- ⋈ Exch. Reg. w/t mean
- ⋈ Exch. Reg.
- Exch. Cov. MM
- ◆ Exch. Cov. w/ mean
- ★ **Exch. Cov.**

# Law Enforcement

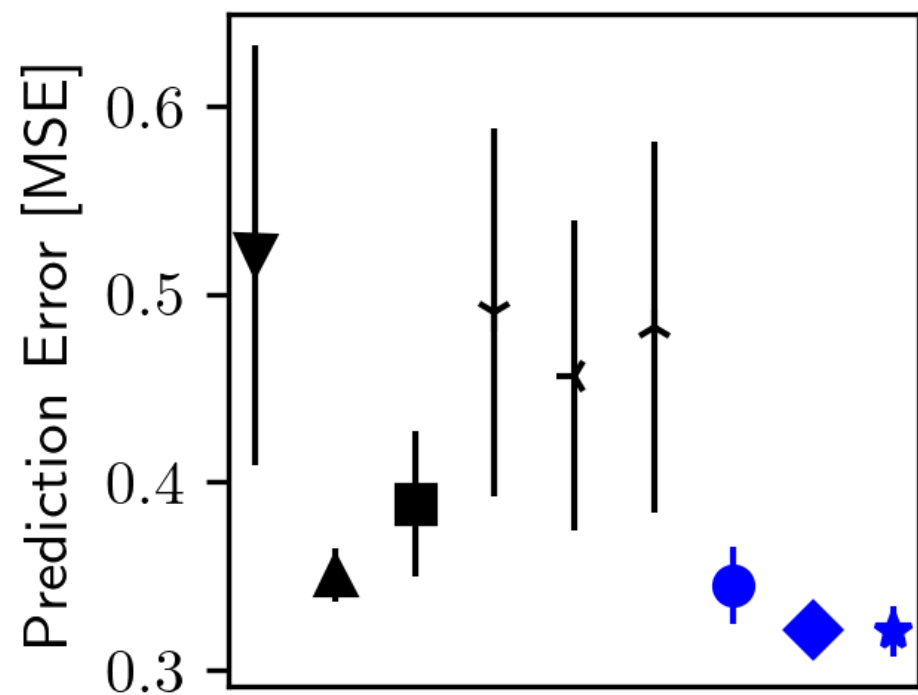

# Blogs

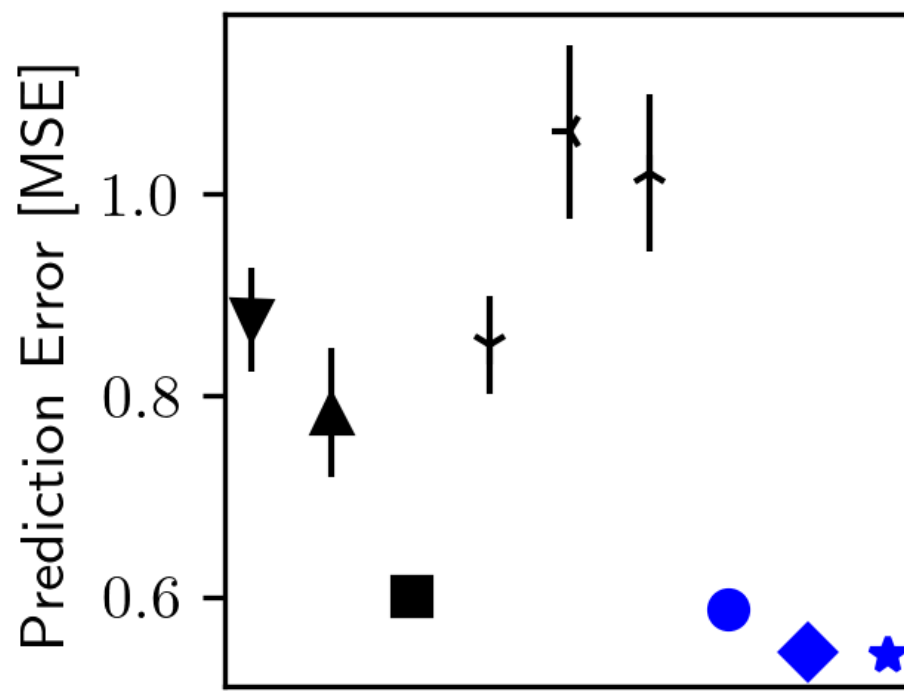

- ▼ Least Sqr./MLE
- ▲ Least Sqr./MLE Pool
- Indep. Bayes.
- ⋈ Exch. Data MM
- ⋈ Exch. Data w/t mean
- ⋈ Exch. Data
- Exch. Cov. MM
- ◆ Exch. Cov. w/ mean
- ★ **Exch. Cov.**
